# Supplementary material for: Deriving the Probabilistic Capacity of General Run-Length Sets Using Generating Functions
Source: arXiv:1001.2205 source file (2010-01-13)
Supplement: Supplementary file 1 [file appendix.tex]

\section{Discussion of \cite{Yeung2009}}

\subsection{Generating Functions}

The authors of \cite{Yeung2009} do not derive the complete generating function of constrained run-lenths.

\subsection{Combinatorial Capacity}
Define 
\begin{align}
N_\delta(T)=|\{a\in A\;|\;w(a)\leq T \text{ and } T-w(a)<\delta\}|
\end{align}
\begin{align}
\mathsf{C}_\delta &= \limsup_{k\rightarrow\infty}\dfrac{\ln N_\delta(\nu_k)}{\nu_k}
\end{align}
This definition leads to the same value for the capacity as our definition. For every $\nu_k$, there is a $T_k\leq\nu_k$ such that
\begin{align}
\sum\limits_{l\leq k}N(\nu_k)\geq N(T_k)\geq \frac{1}{\lceil\frac{\nu_k}{\nu_1}\rceil}\sum\limits_{l\leq k}N(\nu_k)
\end{align}
The penalty factor $\lceil\nu_k/\nu_1\rceil^{-1}$ increases only linear in $\nu_k$, so in the limit $\mathsf{C}_\delta=\mathsf{C}$.

\subsection{Probabilistic Capacity}

The authors in \cite{Yeung2009} use a different definition of entropy rate. Basically, they define a random variable $X^{T}$ with the support $\mathcal{X}^{T}=\{a\in\mathcal{A}\,\vert\,w(a)\leq T\}$ and define the probabilistic capacity $\mathsf{R}_T$ as
\begin{align}
\mathsf{R}_T = \max_{p_{X_T}}\lim_{T\rightarrow\infty} \frac{\entop(X^T)}{T}
\end{align}
For this definition, it is easy to show that $\mathsf{R}_T\leq \mathsf{C}$: it directly follows from $\entop(X^{T})\leq \ln\lvert\mathcal{X}^T\rvert$. However, it is difficult to show that a stochastic process reaches $\mathsf{C}$. With our definition, it is the other way round: it is intricate to show that $\mathsf{R}\leq\mathsf{C}$ holds for any constrained systems, but this bound is established in Theorem~\ref{theo:inputProcess}. It is now straight-forward to show for a specific constrained system that a stochastic process reaches the bound.
